# Supplementary material for: Characterizing the Interplay between Polymer Solvation and Conformation
Source: arXiv:2103.07630 source file (2021-03-13)
Supplement: Supplementary file 1 [file suppl_poly_March1_AJP.pdf]

# Supplementary Material

## Characterizing the Interplay between Polymer Solvation and Conformation

Debdas Dhabal, Zhitong Jiang and Amish J. Patel*

Department of Chemical and Biomolecular Engineering, University of Pennsylvania, Philadelphia, Pennsylvania 19104, United States

Three supplementary figures, which support the results presented in the main text are included.

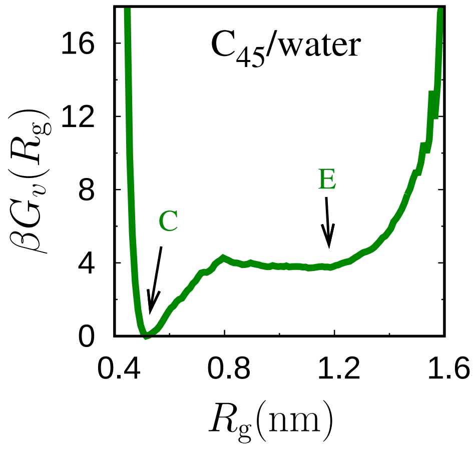


**Figure S1** For the $C_{45}$ polymer in water, the conformational free energy landscape, $G_v(R_g)$, obtained by integrating $\exp[-\beta G_v(\tilde{N}, R_g)]$ over the solvent coordinate, $\tilde{N}$, is shown as a function of the polymer radius of gyration, $R_g$. The basins corresponding to collapsed (C) and extended (E) states are denoted by arrows.

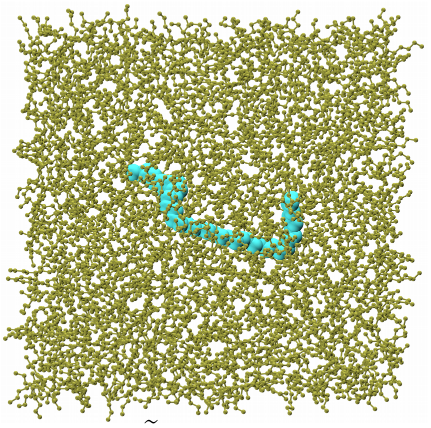

$\tilde{N}_v \approx 269$

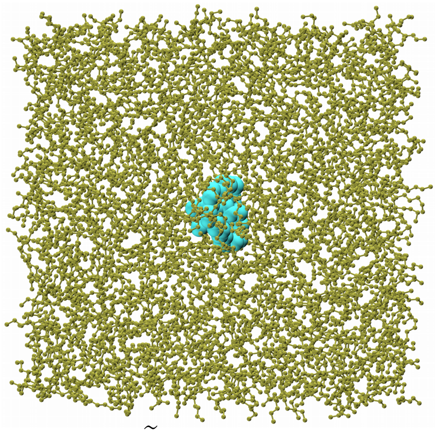

$\tilde{N}_v \approx 142$

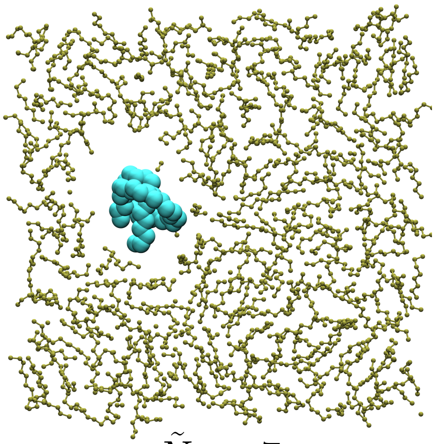

$\tilde{N}_v \approx 7$

**Figure S2** Simulation snapshots of the $C_{45}$ polymer (beads shown in cyan using spacefill representation) solvated in octane (gold) are shown for three select $\tilde{N}_v$-values. As shown in the topmost snapshot, the polymer adopts an extended configuration for $\tilde{N}_v > \langle \tilde{N}_v \rangle_{\phi_1^*}$. The middle snapshot highlights that the polymer is in a collapsed, but solvated configuration for $\langle \tilde{N}_v \rangle_{\phi_2^*} < \tilde{N}_v < \langle \tilde{N}_v \rangle_{\phi_1^*}$. Finally, the bottom snapshot indicates that the collapsed polymer is dewetted for $\tilde{N}_v < \langle \tilde{N}_v \rangle_{\phi_2^*}$; solvent beads in the background are hidden to clearly illustrate polymer dewetting.

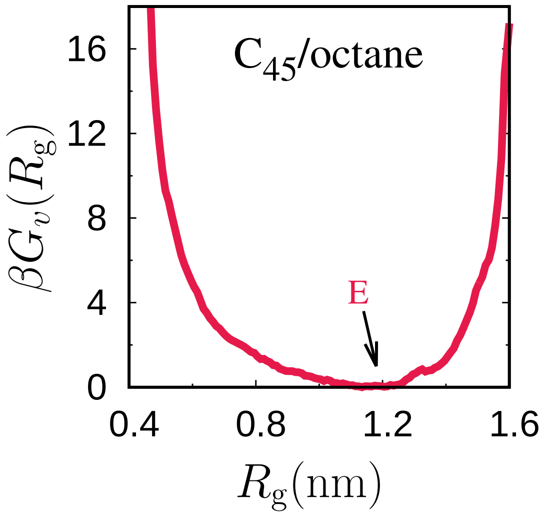


**Figure S3** For the $C_{45}$ polymer in octane, the conformational free energy landscape, $G_v(R_g)$, obtained by integrating $\exp[-\beta G_v(\tilde{N}, R_g)]$ over the solvent coordinate, $\tilde{N}$, is shown as a function of the polymer radius of gyration, $R_g$. The basins corresponding to the extended (E) state is denoted by an arrow; no distinct basin is observed for the collapsed state.
